# Supplementary material for: Contractile stresses in cohesive cell layers on finite-thickness substrates
Source: arXiv:1204.3019 ancillary file (2012-07-18)
Supplement: Supplementary file 1 [file SupplementalMaterial.pdf]

# Contractile stresses in cohesive cell layers on finite-thickness substrates
# Supplemental Material

Shiladitya Banerjee and M. Cristina Marchetti
(Dated: June 5, 2012)

## I. GREEN'S FUNCTION FOR ELASTIC SUBSTRATE OF FINITE THICKNESS

Here we outline the derivation of the Green's function at the surface of the elastic substrate using Fourier techniques. We assume that the substrate is an isotropic and homogeneous elastic material in two dimensions, with Young's modulus $E$ [1] and Poisson ratio $\nu_s$. The substrate displacement field is denoted by $\mathbf{v}$. In the plane stress approximation, the constitutive relation for the substrate stress is given as,

$$\sigma^s_{ij} = \frac{E}{1+\nu_s}\left[\frac{\nu_s}{1-\nu_s}\nabla.\mathbf{v}\;\delta_{ij} + \frac{1}{2}\left(\partial_i v_j + \partial_j v_i\right)\right] . \tag{1.1}$$

In equilibrium, the substrate deformations $\mathbf{v}$ are governed by the standard equation of elastostatics for plane stress deformations,

$$\left(\frac{1-\nu_s}{1+\nu_s}\right)\nabla^2\mathbf{v} + \nabla(\nabla.\mathbf{v}) = 0 . \tag{1.2}$$

Turning to boundary conditions, we assume that there are negligible normal stresses at the substrate surface letting $\sigma^s_{zz}(z = h_s) = 0$. Assuming that the substrate is plated on a rigid surface, displacements at the bottom of the substrate are zero, $\mathbf{v}(z = 0) = 0$. The $x-$displacements at the top layer of the substrate, denoted by $u^s(x) = v_x(x, z = h_s)$, can then be written in terms of the Green's function of Eq. (1.2) as,

$$u^s(x) = \int_{x'} G(|x - x'|)\sigma^s_{xz}(x', z = h_s) . \tag{1.3}$$

The shear stress at the cell-substrate interface $\sigma^s_{xz}(x)|_{z=h_s}$, represents the traction stress exerted by the adherent cell. Working in Fourier space with respect to $x$, we write all functions as $f(x,z) = \int_{-\infty}^{\infty} dq f(q,z)e^{\imath qx}$. Eq.(1.2) then becomes,

$$\left(\frac{1-\nu_s}{1+\nu_s}\right)\partial_z^2 v_x + \imath q\partial_z v_z - \left(\frac{2}{1+\nu_s}\right)q^2 v_x = 0 , \tag{1.4a}$$

$$\left(\frac{2}{1+\nu_s}\right)\partial_z^2 v_z + \imath q\partial_z v_x - \left(\frac{1-\nu_s}{1+\nu_s}\right)q^2 v_z = 0 . \tag{1.4b}$$

Eqs. (1.4a) and (1.4b) can now be conveniently solved for $\mathbf{v}$ with the given boundary conditions. In particular we seek the traction stress at the cell-substrate interface given by $T_x(q) = \sigma_{xz}(q, z = h_s)$ as a function of $u^s_x$. The final result can be compactly written as, $T_x(q) = Q(q)u^s(q)$, where

$$Q(q) = \mu q\frac{(3-\nu_s)(1+\nu_s)(e^{4h_s q}+1) + 2e^{2h_s q}\left[(5-2\nu_s+\nu_s^2) + 2h_s^2q^2(1+\nu_s)^2\right]}{(3-\nu_s)(e^{4h_s q}-1) + 4e^{2h_s q}h_s q(1+\nu_s)} , \tag{1.5}$$

where $\mu = E/2(1 + \nu_s)$ is the shear modulus of the substrate. The stiffness function $Q(q)$ is related to the Green's function for the surface substrate as,

$$G(x) = \frac{1}{2\pi}\int dq\; Q^{-1}(q)e^{-\imath qx} . \tag{1.6}$$

For long wavelengths $qh_s \ll 1$, which corresponds to a thin substrate, we get $Q(q) \to \mu/h_s$. The Green's function is then given by,

$$G(x) = \frac{h_s}{\mu}\delta(x) . \tag{1.7}$$

For short wavelengths $qh_s \gg 1$, corresponding to an elastic half-plane we obtain $Q(q) \to \mu q(1+\nu_s)$, and the Green's function is given by

$$G(|x|) = -\frac{2}{\pi E}\left[\gamma + \log\left(|x|/L\right)\right] \; . \tag{1.8}$$

For an elastic slab of finite thickness we use the following approximate form interpolating between the limits of thin and infinitely thick substrates,

$$Q \simeq \frac{\mu}{h_s}\sqrt{1+\left[qh_s(1+\nu_s)\right]^2} \; . \tag{1.9}$$

Fig. 1 shows a comparison between the exact stiffness function given in Eq. (1.5) and the interpolated form given in Eq. (1.9). Using Eq. (1.9) we can perform the Fourier inversion analytically to obtain the Green's function in real space in terms of a modified Bessel function of the second kind, as

$$G(x) = \frac{2}{\pi E} K_0\left[\frac{|x|}{h_s(1+\nu_s)}\right] \; . \tag{1.10}$$

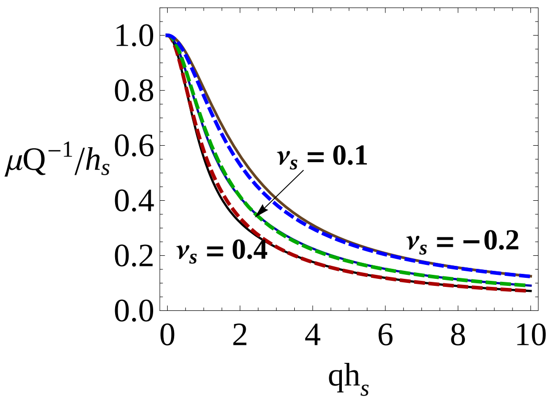


FIG. 1: The inverse local stiffness $Q^{-1}\mu/h_s$ as a function of wavenumber $qh_s$, comparing the exact solution in Eq. (1.5) (solid lines) with the approximate form in Eq. (1.9) (dashed lines). Poisson ratios : $\nu_s = 0.1$ (green), $\nu_s = 0.4$ (red), $\nu_s = -0.2$ (blue).

## II. ONE DIMENSIONAL CELL LAYER ON ELASTIC HALF PLANE

In this section we derive the solution for the internal stress distribution in a one-dimensional cell layer adhering to an elastic half plane, using the Green's function given by Eq. (1.8). The stress $\sigma(x)$ obeys the integro-differential equation,

$$\ell_a^2 \partial_x^2 \sigma + \sigma_a = \sigma + \frac{\ell_{s\infty}^2}{2L}\,\text{p.v.}\int_0^L dx' \frac{\sigma'(x')}{x-x'} \; , \tag{2.1}$$

where, $\ell_{s\infty} = \sqrt{4B_c h_c L/\pi E_s}$ and p.v. denotes principal value. We then expand $\sigma(x)$ in a Fourier sine series as $\sigma(x) = \sum_{n=1}^{\infty} \sigma_n \sin\left(n\pi x/L\right)$, which satisfies the boundary condition $\sigma|_{x=0} = \sigma|_{x=L} = 0$. Eq (2.1) then becomes,

$$\sigma_a = \sum_{n=1}^{\infty} \sigma_n \sin\left(\hat{n}x\right)\left[\hat{n}^2\ell_a^2 + 1\right] + \frac{\ell_{s\infty}^2}{2L}\sum_{m=1}^{\infty} \hat{m}\sigma_m \int_0^L dx' \frac{\cos\left(\hat{m}x'\right)}{x-x'} \; , \tag{2.2}$$

where $\hat{n} = n\pi/L$. We then integrate both sides of Eq. (2.2) by $\frac{2}{L}\int_0^L dx \sin\left(\hat{n}x\right)$ to reduce Eq. (2.1) to a linear system of algebraic equations for the Fourier mode amplitudes, $\sigma_n$, given by

$$\frac{2(1-(-1)^n)}{n\pi}\sigma_a = \left(1+\ell_a^2\hat{n}^2\right)\sigma_n + \left(\frac{\ell_{s\infty}}{L}\right)^2 \sum_{m=1}^{\infty} H_{mn}\sigma_m \; , \tag{2.3}$$

where the dimensionless mode coupling matrix $H_{mn}$ is given by,

$$H_{mn} = m\pi \int_0^1 dx' \int_0^1 dx \; \sin(n\pi x) \frac{1}{x - x'} \cos(m\pi x') \; . \tag{2.4}$$

$H_{mn}$ can be analytically or numerically evaluated after regularizing the integral by providing a short-distance cut-off $a$ as introduced earlier. Using computed values for $H_{mn}$, we solve numerically for the Fourier amplitudes $\sigma_n$, and then obtain $\sigma(x)$ by summing a series.

## III. TWO DIMENSIONAL CELL LAYERS

For completeness we show here that the elastic deformation of a planar cell layer adhering to a two-dimensional substrate can also be described by a single equation for the thickness-averaged stress tensor of the cellular material, although in general shear and compressional deformations are coupled. The case of a circular cell layer where spatial variation only occur along the radial direction can again be reduced to a one-dimensional problem and was discussed in Ref. [10] of the Letter for the case of infinitely thin substrate. The case of a circular cell on a substrate of arbitrary thickness will be addressed in a future publication.

Considering a cell layer in the $xy$ plane of thickness $h_c$ in the $z$ direction, with $h_c$ small compared to the lateral dimension $L$ of the layer, the force balance equation, averaged over the cell thickness, is

$$Y_a \left[ u_i(\mathbf{x}) - u_i^s(\mathbf{x}) \right] = h_c \partial_j \overline{\sigma}_{ij}(\mathbf{x}) \; , \tag{3.1}$$

where $\mathbf{x}$ is a position in the $xy$ plane, $i, j$ denote in-plane cartesian components, $Y_a$ describes the effective strength of the focal adhesions, $\mathbf{u}(\mathbf{x})$ is the two-dimensional displacement field of the cellular medium at $z = h_s$, and $\overline{\sigma}_{ij}$ is the in-plane cellular stress tensor averaged over the thickness of the cell, $\overline{\sigma}_{ij}(\mathbf{x}) = 1/h_c \int_{h_s}^{h_s+h_c} dz \; \sigma_{ij}(\mathbf{x}, z)$, given by $\overline{\sigma}_{ij}(\mathbf{x}) = B_c u_{kk} \delta_{ij} + 2\mu_c \left[ u_{ij} - \delta_{ij} u_{kk} \right] + \sigma_a \delta_{ij}$, with $B_c$ and $\mu_c$ the longitudinal and shear elastic moduli of the cell layer and $\sigma_a$ is the isotropic active stress. Although we have neglected components of the cellular displacements along the cell thickness and spatial variations along $z$, the cell elastic constants are those of a three-dimensional cellular medium. The substrate deformation at the surface is

$$u_i^s(\mathbf{x}) = h_c \int d\mathbf{x}' G_{ij}(\mathbf{x} - \mathbf{x}') \partial_k' \overline{\sigma}_{jk}(\mathbf{x}') \; , \tag{3.2}$$

with $\mathbf{G}$ the elastic Green's tensor of a substrate of infinite extent in the $xy$ plane, occupying the region $0 \le z \le h_s$, evaluated at $z = h_s$. Eqs. (3.1)-(3.2) can be reduced to integro-differential equations for the cellular stress, as

$$\ell_a^2 \left[ \partial_i \partial_k \overline{\sigma}_{kj} \right]^S + \delta_{ij} \sigma_a = \overline{\sigma}_{ij} + \frac{2\mu_c}{B_c - 2\mu_c} \delta_{ij} \left( \overline{\sigma}_{kk} - 2\sigma_a \right) - (B_c + 2\mu_c) h_c \int d\mathbf{x}' \left[ \partial_i \partial_l G_{ik}(\mathbf{x} - \mathbf{x}') \overline{\sigma}_{kl}(\mathbf{x}') \right]^S \; , \tag{3.3}$$

where, $\ell_a = \sqrt{(B_c + 2\mu_c) h_c / Y_a}$, and $[...]^S$ denotes symmetrization with respect to indices that are not summed over, e.g., $\left[ \partial_i \partial_k \overline{\sigma}_{kj} \right]^S = \frac{1}{2} \left[ \partial_i \partial_k \overline{\sigma}_{kj} + \partial_j \partial_k \overline{\sigma}_{ki} \right]$. The one dimensional case can then be obtained by letting $\mu_c = 0$ and considering only spatial variations along $x$.

---

[1] The Young modulus $E$ of an elastic sheet has dimensions of force per unit length. In the main text we express our results in terms of the Young modulus $E_s$ of a three dimensional elastic medium, with dimensions of force per unit area. The reason for this choice is to express the various length scales in terms of experimentally accessible quantities. In general the two quantities can be related via a length scale $d$ as $E = E_s d$, with $d$ describing the thickness of the substrate in the $y$ direction normal to the direction of linear extent of the putative one-dimensional cell. We choose $d = \ell_{c0}$ when describing an individual cell and $d = L$ when describing a cell layer. The results do not depend on this length.
